# Supplementary material for: Low-frequency excess vibrational modes in two-dimensional glasses
Source: arXiv:2107.01505 source file (2021-07-03)
Supplement: Supplementary file 1 [file SM-V02.pdf]

# Supplemental Material: Low-frequency excess vibrational modes in two-dimensional glasses

Lijin Wang[1], Grzegorz Szamel[2], and Elijah Flenner[2]
[1]School of Physics and Materials Science, Anhui University, Hefei 230601, P. R. China and
[2]Department of Chemistry, Colorado State University, Fort Collins, Colorado 80523, USA

In the supplemental material, we first describe the simulation details of the four model glass formers where we produce results presented in the main text, and then show further results to support some of our descriptions in the main text.

## I. SIMULATIONS

Our each simulated 2D model is composed of $N$ discs with equal mass $m$. Periodic boundary conditions are applied in all directions in all model glasses examined.

Our IPL-12 model and IPL-10 model are the purely repulsive inverse power law potential models with different simulation parameters, and hence we describe the two models together. In the inverse power law potential, the interaction between two particles $i$ and $j$ with the separation $r_{ij}$ is given by $V_{IPL}(r_{ij}) = [\left(\frac{\sigma_{ij}}{r_{ij}}\right)^n + c_0 + c_2\left(\frac{r_{ij}}{\sigma_{ij}}\right)^2 + c_4\left(\frac{r_{ij}}{\sigma_{ij}}\right)^4)]H(r_{ij}^c - r_{ij})$, where $H(r)$ is the Heaviside step function, and the constants $c_0$, $c_2$ and $c_4$ are chosen to make $V(r_{ij})$ and its first and second derivatives continuous at the interaction cutoff $r_{ij}^c$.

In our 2D *IPL-12 model* [1], the exponent $n = 12$ in $V_{IPL}(r_{ij})$ and the interaction cutoff $r_{ij}^c = 1.25\sigma_{ij}$. We use a continuous size polydispersity with the probability distribution of particle diameters $\sigma \in [0.73, 1.62]$ following $F(\sigma) \sim \frac{1}{\sigma^3}$; the cross-diameter $\sigma_{ij}$ obeys a non-additive mixing rule, $\sigma_{ij} = \frac{\sigma_i+\sigma_j}{2}(1 - \lambda|\sigma_i - \sigma_j|)$ with $\lambda = 0.2$. We performed simulations in this model system at the number density $\rho = 1.0$ and different parent temperatures $T_p$ ranging from $T_p = 0.400$ to $T_p = 0.030$.

In our 2D *IPL-10 model* [2], $n = 10$ in $V_{IPL}(r_{ij})$ and $r_{ij}^c = 1.48\sigma_{ij}$. This model system is composed of a 50:50 binary mixture of $A$ discs and $B$ discs. Here, we set $\sigma_{AA} = 1.0$, $\sigma_{BB} = 1.4$, and $\sigma_{AB} = 1.18$. High-temperature equilibrated configurations in this model were created at $T_p = 2.0$ and $\rho = 0.86$.

Our 2D *LJ-12 model* [3] is the Lennard-Jones potential system filled with two types of discs: $A$ discs and $B$ discs. The number ratio of $A$ discs to $B$ disc is $65 : 35$. The interaction between two discs $i$ and $j$ is $V_{LJ}(r_{ij}) = [f(r_{ij}) - f(r_{ij}^c) - (r_{ij} - r_{ij}^c)f'(r_{ij}^c)]H(r_{ij}^c - r_{ij})$, where $f(r_{ij}) = 4\epsilon_{ij}[\left(\frac{\sigma_{ij}}{r_{ij}}\right)^{12} - \left(\frac{\sigma_{ij}}{r_{ij}}\right)^6]$, $H(r)$ is the Heaviside step function, and $r_{ij}^c = 2.5\sigma_{ij}$. Here, $\sigma_{AA} = 1.0$, $\sigma_{BB} = 0.88$, $\sigma_{AB} = 0.8$,$\epsilon_{AA} = 1.0$, $\epsilon_{BB} = 0.5$, and $\epsilon_{AB} = 1.5$. Our equilibrated configurations in this model system were obtained at $T_p = 6.0$ and $\rho = 1.2$.

In our 2D *HARM model* , the interaction between two particles $i$ and $j$ is the purely repulsive harmonic potential $V_{HARM}(r_{ij}) = (1 - r_{ij}/\sigma_{ij})^2/2$ when their separation $r_{ij}$ is smaller than $\sigma_{ij} = 0.5(\sigma_i + \sigma_j)$, and zero otherwise. Our model system is composed of a 50:50 binary mixture of $A$ and $B$ discs. Here, $\sigma_A = 1.4$ and $\sigma_B = 1.0$. We got equilibrated configurations in this model system at $T_p = 0.1$ and $\rho = 0.946$.

## II. FURTHER RESULTS

In Fig. 1 we show the ensemble size dependence of the total cumulative density of states $I(\omega)$ in the 2D IPL-12 model system with $N = 1000$. For the same data, we also show the plot of $I(\omega)/\omega^4$ vs. $\omega$ in the inset. Our maximum ensemble size in this system is around 2.2 million. It can be seen the results do not depend on ensemble size examined here.

Figure 2 shows $I(\omega)/\omega^4$ and $I(\omega)/\omega^5$ against $\omega$ for the same data as presented in Fig.3 in the main text. An approximate plateau in the $I(\omega)/\omega^4$ plot but not $I(\omega)/\omega^5$ plot at very low frequencies in each model can be observed, further suggesting $I(\omega) \sim \omega^4$ should be the correct scaling.

Figure 3 demonstrates that there is an overlapping frequency region where the $\omega^3$ scaling is followed by the cumulative density of excess modes $I_{\rm exc}(\omega)$ determined by subtracting off the Debye contribution and where the $\omega^4$ scaling is followed by the cumulative density of all modes in very small systems.

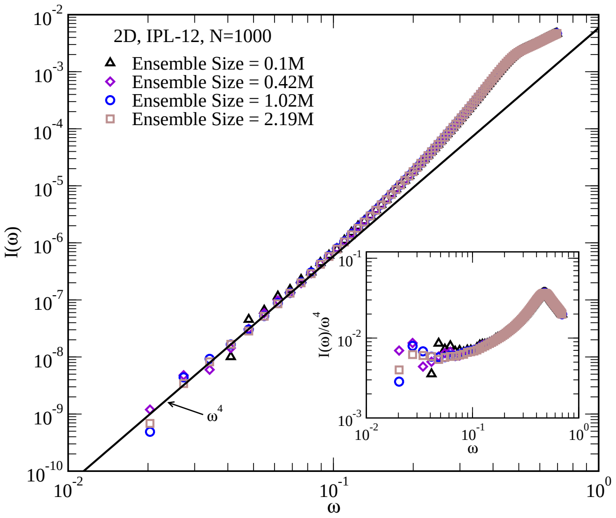


FIG. 1: Ensemble size dependence of the total cumulative density of states $I(\omega)$ at $T_p = 0.400$ for $N = 1000$ system in the 2D IPL-12 model. The solid line represents $I(\omega) \sim \omega^4$. (Inset) The same data plotted as $I(\omega)/\omega^4$ against $\omega$.

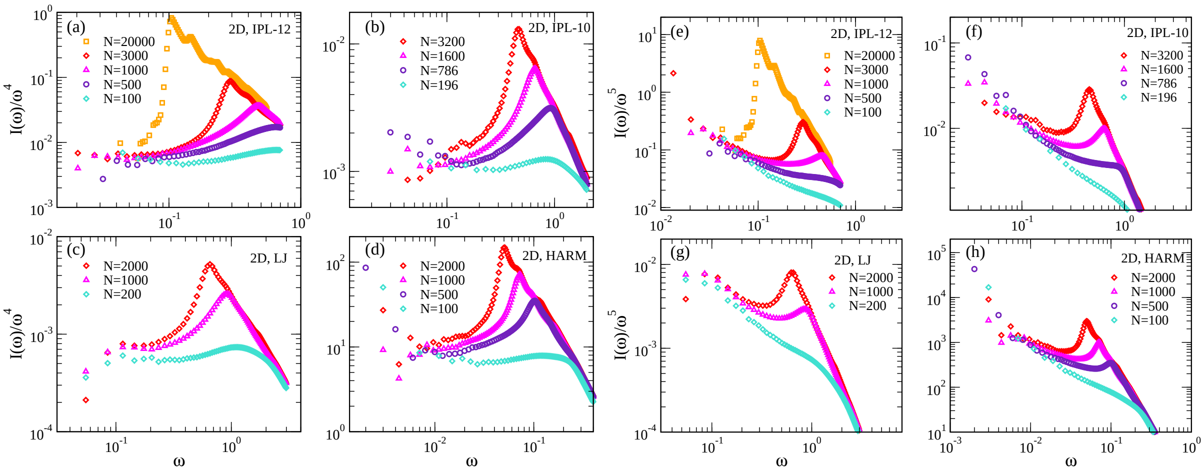


FIG. 2: The reduced total cumulative density of states $I(\omega)/\omega^4$ and $I(\omega)/\omega^5$ in small systems in the 2D IPL-12 model [(a) and (e)], 2D IPL-10 model [(b) and (f)], 2D LJ model [(c) and (g)], and 2D HARM model [(d) and (h)].

[1] L. Berthier, P. Charbonneau, A. Ninarello, M. Ozawa, and S. Yaida, Nat. Commun. **10**, 1508 (2020).
[2] G. Kapteijns, E. Bouchbinder, and E. Lerner, J. Chem. Phys. **148**, 214502 (2018).
[3] R. Bruning, D. A. St-Onge, S. Patterson, and W. Kob, J. Phys.: Condens. Matter **21**, 035117 (2009).
[4] C. S. O'Hern, L. E. Silbert, A. J. Liu, and S. R. Nagel, Phys. Rev. E **68**, 011306 (2003).

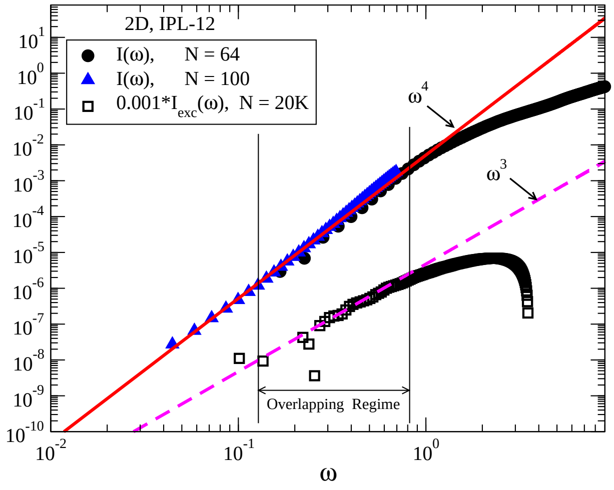


FIG. 3: Comparison of the cumulative density of states of excess modes $I_{\rm exc}(\omega)$ calculated by subtracting off the Debye contribution (see Eq.1 in the main text) in $N = 20000$ system and the total cumulative density of states $I(\omega)$ in $N = 64$ and 100 systems at $T_p = 0.400$ in the 2D IPL-12 model. Dashed and solid lines correspond to $I_{\rm exc}(\omega) \sim \omega^3$ and $I(\omega) \sim \omega^4$, respectively. One can see there is an overlapping frequency range (indicated by the horizontal line with arrows in both ends) where $I_{\rm exc}(\omega)$ scales as $\omega^3$ and where $I(\omega)$ scales as $\omega^4$. $I_{\rm exc}(\omega)$ is rescaled by a factor of 0.001 for visualization purpose.
